# Supplementary material for: Efficient Generation of Parameterised Quantum Circuits from Large Texts
Source: arXiv:2505.13208 source file (2025-05-19)
Supplement: Supplementary file 2 [file conj2.tex]

\documentclass{standalone}
\usepackage{tikz}

\begin{document}
\tikzset{every picture/.style={line width=0.75pt}, anchor=base} %set default line width to 0.75pt

\tikzstyle{black_wire}=[-, draw={rgb,255: red,0; green,0; blue,0}, line width=1.0pt]
\tikzstyle{box}=[-, fill={rgb,255: red,255; green,255; blue,255}, line width=1.0pt]
\tikzstyle{dotted_box}=[-, dash pattern={on 0.84pt off 2.51pt}, fill={rgb,255: red,255; green,255; blue,255}, line width=1.0pt]
\tikzstyle{spider}=[circle, fill=black, minimum size=3pt, inner sep=0.5ex]

% When embedding into a *.tex file, uncomment and include the following lines:
\pgfdeclarelayer{nodelayer}
\pgfdeclarelayer{edgelayer}
\pgfdeclarelayer{labellayer}
\pgfsetlayers{nodelayer, edgelayer, labellayer}
\begin{tikzpicture}
	\begin{pgfonlayer}{nodelayer}
		\node [] (1) at (4, 1.5) {};
		\node [] (2) at (4, 1.25) {};
		\node [] (3) at (6, 1.5) {};
		\node [] (4) at (6, 1.25) {};
		\node [] (5) at (12.5, 1.5) {};
		\node [] (6) at (12.5, 1.25) {};
		\node [] (7) at (14.5, 1.5) {};
		\node [] (8) at (14.5, 1.25) {};
		\node [] (9) at (10.2143, 2.1) {};
		\node [] (10) at (10.2143, 1.25) {};
		\node [] (11) at (11.5, 1.5) {};
		\node [] (12) at (11.5, 1.25) {};
		\node [] (13) at (9.80357, 1.825) {};
		\node [] (14) at (9.80357, 1) {};
		\node [] (15) at (12, 1.5) {};
		\node [] (16) at (12, 1) {};
		\node [] (17) at (3.5, 1.5) {};
		\node [] (18) at (3.5, 1) {};
		\node [] (19) at (7.78571, 2.1) {};
		\node [] (20) at (7.78571, 1) {};
		\node [] (21) at (3, 1.5) {};
		\node [] (22) at (3, 1) {};
		\node [] (23) at (8.19643, 1.825) {};
		\node [] (24) at (8.19643, 1) {};
		\node [] (25) at (1, 1.5) {};
		\node [] (26) at (1, 1) {};
		\node [] (27) at (8.60714, 1.7) {};
		\node [] (28) at (8.60714, 1) {};
		\node [] (29) at (9.39286, 1.7) {};
		\node [] (30) at (9.39286, -2) {};
		\node [] (31) at (5, 0.925) {};
		\node [] (32) at (13.5, 1) {};
		\node [] (33) at (10.8571, 1) {};
		\node [] (34) at (10.9643, 0.425) {};
		\node [] (35) at (5.64286, 0.4) {};
		\node [] (36) at (5.53571, -0.05) {};
		\node [] (37) at (4.67857, -0.6) {};
		\node [] (38) at (0, 1.5) {};
		\node [] (39) at (2, 1.5) {};
		\node [] (40) at (2, 2) {};
		\node [] (41) at (1, 2.1) {};
		\node [] (42) at (0, 2) {};
		\node [] (44) at (2.5, 1.5) {};
		\node [] (45) at (4.5, 1.5) {};
		\node [] (46) at (4.5, 2) {};
		\node [] (47) at (3.5, 2.1) {};
		\node [] (48) at (2.5, 2) {};
		\node [] (50) at (5, 1.5) {};
		\node [] (51) at (7, 1.5) {};
		\node [] (52) at (7, 2) {};
		\node [] (53) at (6, 2.1) {};
		\node [] (54) at (5, 2) {};
		\node [] (56) at (7.5, 1.5) {};
		\node [] (57) at (10.5, 1.5) {};
		\node [] (58) at (10.5, 3) {};
		\node [] (59) at (9, 3.1) {};
		\node [] (60) at (7.5, 3) {};
		\node [] (62) at (11, 1.5) {};
		\node [] (63) at (13, 1.5) {};
		\node [] (64) at (13, 2) {};
		\node [] (65) at (12, 2.1) {};
		\node [] (66) at (11, 2) {};
		\node [] (68) at (13.5, 1.5) {};
		\node [] (69) at (15.5, 1.5) {};
		\node [] (70) at (15.5, 2) {};
		\node [] (71) at (14.5, 2.1) {};
		\node [] (72) at (13.5, 2) {};
		\node [] (75) at (9.61071, 2.05) {};
		\node [] (76) at (8.38929, 2.05) {};
		\node [] (77) at (9, 2.1) {};
		\node [] (78) at (8.39286, 2.3) {};
		\node [] (79) at (9.60714, 2.3) {};
	\end{pgfonlayer}
	\begin{pgfonlayer}{edgelayer}
		\draw [style={dotted_box}] (56.center)
			 to (57.center)
			 to (58.center)
			 to (59.center)
			 to (60.center)
			 to cycle;
		\draw [style={black_wire}, in=90, out=-90] (1.center) to (2.center);
		\draw [style={black_wire}, in=90, out=-90] (3.center) to (4.center);
		\draw [style={black_wire}, in=90, out=-90] (5.center) to (6.center);
		\draw [style={black_wire}, in=90, out=-90] (7.center) to (8.center);
		\draw [style={black_wire}, in=90, out=-90] (9.center) to (10.center);
		\draw [style={black_wire}, in=90, out=-90] (11.center) to (12.center);
		\draw [style={black_wire}, in=90, out=-90] (13.center) to (14.center);
		\draw [style={black_wire}, in=90, out=-90] (15.center) to (16.center);
		\draw [style={black_wire}, in=90, out=-90] (17.center) to (18.center);
		\draw [style={black_wire}, in=90, out=-90] (19.center) to (20.center);
		\draw [style={black_wire}, in=90, out=-90] (21.center) to (22.center);
		\draw [style={black_wire}, in=90, out=-90] (23.center) to (24.center);
		\draw [style={black_wire}, in=90, out=-90] (25.center) to (26.center);
		\draw [style={black_wire}] (27.center) to (28.center);
		\draw [style={black_wire}, in=90, out=-90] (29.center) to (30.center);
		\draw [style={black_wire}, in=180, out=-90, looseness=0.75] (2.center) to (31.center);
		\draw [style={black_wire}, in=0, out=-90, looseness=0.75] (4.center) to (31.center);
		\draw [style={black_wire}, in=180, out=-90, looseness=0.75] (6.center) to (32.center);
		\draw [style={black_wire}, in=0, out=-90, looseness=0.75] (8.center) to (32.center);
		\draw [style={black_wire}, in=180, out=-90] (10.center) to (33.center);
		\draw [style={black_wire}, in=0, out=-90] (12.center) to (33.center);
		\draw [style={black_wire}, in=180, out=-90, looseness=1.25] (14.center) to (34.center);
		\draw [style={black_wire}, in=0, out=-90, looseness=1.25] (16.center) to (34.center);
		\draw [style={black_wire}, in=180, out=-90, looseness=0.75] (18.center) to (35.center);
		\draw [style={black_wire}, in=0, out=-90, looseness=0.75] (20.center) to (35.center);
		\draw [style={black_wire}, in=180, out=-90] (22.center) to (36.center);
		\draw [style={black_wire}, in=0, out=-90] (24.center) to (36.center);
		\draw [style={black_wire}, in=180, out=-90] (26.center) to (37.center);
		\draw [style={black_wire}, in=0, out=-90] (28.center) to (37.center);
		\draw [style=box] (38.center)
			 to (39.center)
			 to (40.center)
			 to (41.center)
			 to (42.center)
			 to cycle;
		\draw [style=box] (44.center)
			 to (45.center)
			 to (46.center)
			 to (47.center)
			 to (48.center)
			 to cycle;
		\draw [style=box] (50.center)
			 to (51.center)
			 to (52.center)
			 to (53.center)
			 to (54.center)
			 to cycle;
		\draw [style=box] (62.center)
			 to (63.center)
			 to (64.center)
			 to (65.center)
			 to (66.center)
			 to cycle;
		\draw [style=box] (68.center)
			 to (69.center)
			 to (70.center)
			 to (71.center)
			 to (72.center)
			 to cycle;
		\draw [style={black_wire}, in=180, out=90, looseness=1.25] (29.center) to (75.center);
		\draw [style={black_wire}, in=0, out=90] (13.center) to (75.center);
		\draw [style={black_wire}, in=180, out=90] (23.center) to (76.center);
		\draw [style={black_wire}, in=0, out=90, looseness=1.25] (27.center) to (76.center);
		\draw [style={black_wire}, in=180, out=90, looseness=0.75] (19.center) to (78.center);
		\draw [style={black_wire}, in=0, out=90, looseness=0.75] (77.center) to (78.center);
		\draw [style={black_wire}, in=180, out=90, looseness=0.75] (77.center) to (79.center);
		\draw [style={black_wire}, in=0, out=90, looseness=0.75] (9.center) to (79.center);
		\draw [style={black_wire}, in=0, out=-90] (77.center) to (27.center);
		\draw [style={black_wire}, in=180, out=-90] (77.center) to (29.center);
	\end{pgfonlayer}
    \begin{pgfonlayer}{labellayer}
        \node [style={spider}] (81) at (8.60714, 1.7) {};
		\node [style={spider}] (82) at (9.39286, 1.7) {};
		\node [] (43) at (1, 1.65) {Alice};
		\node [] (49) at (3.5, 1.65) {loves};
		\node [] (55) at (6, 1.65) {music};
		\node [] (67) at (12, 1.65) {plays};
		\node [] (73) at (14.5, 1.65) {piano};
		\node [] (80) at (9, 2.65) {and};
    \end{pgfonlayer}
\end{tikzpicture}
\end{document}
