# Supplementary material for: Efficient Generation of Parameterised Quantum Circuits from Large Texts
Source: arXiv:2505.13208 source file (2025-05-19)
Supplement: Supplementary file 3 [file conj3.tex]

\documentclass{standalone}
\usepackage{tikz}

\begin{document}
\tikzset{every picture/.style={line width=0.75pt}, anchor=base} %set default line width to 0.75pt

\tikzstyle{black_wire}=[-, draw={rgb,255: red,0; green,0; blue,0}, line width=1.0pt]
\tikzstyle{box}=[-, fill={rgb,255: red,255; green,255; blue,255}, line width=1.0pt]
\tikzstyle{dotted_box}=[-, dash pattern={on 0.84pt off 2.51pt}, fill={rgb,255: red,255; green,255; blue,255}, line width=1.0pt]
\tikzstyle{spider}=[circle, fill=black, minimum size=3pt, inner sep=0.5ex]

% When embedding into a *.tex file, uncomment and include the following lines:
\pgfdeclarelayer{nodelayer}
\pgfdeclarelayer{edgelayer}
\pgfdeclarelayer{labellayer}
\pgfsetlayers{nodelayer, edgelayer, labellayer}
\begin{tikzpicture}
	\begin{pgfonlayer}{nodelayer}
		\node [] (1) at (4.5, 1.5) {};
		\node [] (2) at (4.5, 1.25) {};
		\node [] (3) at (6.5, 1.5) {};
		\node [] (4) at (6.5, 1.25) {};
		\node [] (16) at (13, 1) {};
		\node [] (17) at (4, 1.5) {};
		\node [] (18) at (4, 1) {};
		\node [] (25) at (1.5, 1.5) {};
		\node [] (26) at (1.5, 1.25) {};
		\node [] (27) at (3.50714, 1.5) {};
		\node [] (28) at (3.50714, 1.25) {};
		\node [] (29) at (8.5, 0.25) {};
		\node [] (30) at (8.5, -1.5) {};
		\node [] (31) at (5.5, 0.925) {};
		\node [] (34) at (8.5, 0.25) {};
		\node [] (35) at (8.5, 0.25) {};
		\node [] (37) at (2.50357, 0.925) {};
		\node [] (38) at (0.5, 1.5) {};
		\node [] (39) at (2.5, 1.5) {};
		\node [] (40) at (2.5, 2) {};
		\node [] (41) at (1.5, 2.1) {};
		\node [] (42) at (0.5, 2) {};
		\node [] (44) at (3, 1.5) {};
		\node [] (45) at (5, 1.5) {};
		\node [] (46) at (5, 2) {};
		\node [] (47) at (4, 2.1) {};
		\node [] (48) at (3, 2) {};
		\node [] (50) at (5.5, 1.5) {};
		\node [] (51) at (7.5, 1.5) {};
		\node [] (52) at (7.5, 2) {};
		\node [] (53) at (6.5, 2.1) {};
		\node [] (54) at (5.5, 2) {};
		\node [] (81) at (13.5, 1.5) {};
		\node [] (82) at (13.5, 1.25) {};
		\node [] (83) at (15.5, 1.5) {};
		\node [] (84) at (15.5, 1.25) {};
		\node [] (87) at (13, 1.5) {};
		\node [] (88) at (13, 1) {};
		\node [] (89) at (10.5, 1.5) {};
		\node [] (90) at (10.5, 1.25) {};
		\node [] (91) at (12.5071, 1.5) {};
		\node [] (92) at (12.5071, 1.25) {};
		\node [] (93) at (14.5, 0.925) {};
		\node [] (94) at (11.5036, 0.925) {};
		\node [] (95) at (9.5, 1.5) {};
		\node [] (96) at (11.5, 1.5) {};
		\node [] (97) at (11.5, 2) {};
		\node [] (98) at (10.5, 2.1) {};
		\node [] (99) at (9.5, 2) {};
		\node [] (100) at (12, 1.5) {};
		\node [] (101) at (14, 1.5) {};
		\node [] (102) at (14, 2) {};
		\node [] (103) at (13, 2.1) {};
		\node [] (104) at (12, 2) {};
		\node [] (105) at (14.5, 1.5) {};
		\node [] (106) at (16.5, 1.5) {};
		\node [] (107) at (16.5, 2) {};
		\node [] (108) at (15.5, 2.1) {};
		\node [] (109) at (14.5, 2) {};
	\end{pgfonlayer}
	\begin{pgfonlayer}{edgelayer}
		\draw [style={black_wire}, in=90, out=-90] (1.center) to (2.center);
		\draw [style={black_wire}, in=90, out=-90] (3.center) to (4.center);
		\draw [style={black_wire}, in=90, out=-90] (17.center) to (18.center);
		\draw [style={black_wire}, in=90, out=-90] (25.center) to (26.center);
		\draw [style={black_wire}] (27.center) to (28.center);
		\draw [style={black_wire}, in=90, out=-90] (29.center) to (30.center);
		\draw [style={black_wire}, in=180, out=-90, looseness=0.75] (2.center) to (31.center);
		\draw [style={black_wire}, in=0, out=-90, looseness=0.75] (4.center) to (31.center);
		\draw [style={black_wire}, in=0, out=-90, looseness=0.50] (16.center) to (34.center);
		\draw [style={black_wire}, in=180, out=-90, looseness=0.50] (18.center) to (35.center);
		\draw [style={black_wire}, in=180, out=-90, looseness=0.75] (26.center) to (37.center);
		\draw [style={black_wire}, in=0, out=-90, looseness=0.75] (28.center) to (37.center);
		\draw [style=box] (38.center)
			 to (39.center)
			 to (40.center)
			 to (41.center)
			 to (42.center)
			 to cycle;
		\draw [style=box] (44.center)
			 to (45.center)
			 to (46.center)
			 to (47.center)
			 to (48.center)
			 to cycle;
		\draw [style=box] (50.center)
			 to (51.center)
			 to (52.center)
			 to (53.center)
			 to (54.center)
			 to cycle;
		\draw [style={black_wire}, in=90, out=-90] (81.center) to (82.center);
		\draw [style={black_wire}, in=90, out=-90] (83.center) to (84.center);
		\draw [style={black_wire}, in=90, out=-90] (87.center) to (88.center);
		\draw [style={black_wire}, in=90, out=-90] (89.center) to (90.center);
		\draw [style={black_wire}] (91.center) to (92.center);
		\draw [style={black_wire}, in=180, out=-90, looseness=0.75] (82.center) to (93.center);
		\draw [style={black_wire}, in=0, out=-90, looseness=0.75] (84.center) to (93.center);
		\draw [style={black_wire}, in=180, out=-90, looseness=0.75] (90.center) to (94.center);
		\draw [style={black_wire}, in=0, out=-90, looseness=0.75] (92.center) to (94.center);
		\draw [style=box] (95.center)
			 to (96.center)
			 to (97.center)
			 to (98.center)
			 to (99.center)
			 to cycle;
		\draw [style=box] (100.center)
			 to (101.center)
			 to (102.center)
			 to (103.center)
			 to (104.center)
			 to cycle;
		\draw [style=box] (105.center)
			 to (106.center)
			 to (107.center)
			 to (108.center)
			 to (109.center)
			 to cycle;
	\end{pgfonlayer}
    \begin{pgfonlayer}{labellayer}
        \node [style={spider}] (35) at (8.5, 0.25) {};
        \node [] (43) at (1.5, 1.65) {Alice};
		\node [] (49) at (4, 1.65) {loves};
		\node [] (55) at (6.5, 1.65) {music};
		\node [] (110) at (10.5, 1.65) {Alice};
		\node [] (111) at (13, 1.65) {plays};
		\node [] (112) at (15.5, 1.65) {piano};
    \end{pgfonlayer}
\end{tikzpicture}
\end{document}
