# Supplementary material for: Efficient Generation of Parameterised Quantum Circuits from Large Texts
Source: arXiv:2505.13208 source file (2025-05-19)
Supplement: Supplementary file 4 [file conj_base_circuit.tex]

\documentclass{standalone}
\usepackage{tikz}

\begin{document}
% When embedding into a *.tex file, uncomment and include the following lines:
\pgfdeclarelayer{nodelayer}
\pgfdeclarelayer{edgelayer}
\pgfdeclarelayer{labellayer}
\pgfsetlayers{nodelayer, edgelayer, labellayer}
\begin{tikzpicture}[]
\begin{pgfonlayer}{nodelayer}
\node (0) at (0, 0) {};
\node [] (1) at (-0.5, 2.25) {};
\node [] (2) at (0.5, 2.25) {};
\node [] (3) at (0.5, 2.75) {};
\node [] (4) at (-0.5, 2.75) {};
\node [] (6) at (2.0, 2.25) {};
\node [] (7) at (3.0, 2.25) {};
\node [] (8) at (3.0, 2.75) {};
\node [] (9) at (2.0, 2.75) {};
\node [] (11) at (4.5, 2.25) {};
\node [] (12) at (5.5, 2.25) {};
\node [] (13) at (5.5, 2.75) {};
\node [] (14) at (4.5, 2.75) {};
\node [] (16) at (-0.5, 1.25) {};
\node [] (17) at (3.0, 1.25) {};
\node [] (18) at (3.0, 1.75) {};
\node [] (19) at (-0.5, 1.75) {};
\node [] (21) at (2.0, -0.75) {};
\node [] (22) at (5.5, -0.75) {};
\node [] (23) at (5.5, -0.25) {};
\node [] (24) at (2.0, -0.25) {};
\node [] (26) at (0.0, 2.25) {};
\node [] (27) at (0.0, 1.75) {};
\node [] (29) at (2.5, 2.25) {};
\node [] (30) at (2.5, 1.75) {};
\node [] (32) at (0.0, 1.25) {};
\node [] (33) at (0.0, 0.75) {};
\node [] (35) at (2.5, 1.25) {};
\node [] (36) at (2.5, 0.75) {};
\node [] (38) at (2.5, 0.25) {};
\node [] (39) at (2.5, -0.25) {};
\node [] (41) at (5.0, 2.25) {};
\node [] (42) at (5.0, -0.25) {};
\node [] (44) at (0.0, 0.25) {};
\node [] (45) at (0.0, -1.25) {};
\node [] (47) at (2.5, -0.75) {};
\node [] (48) at (2.5, -1.25) {};
\node [] (50) at (0.0, -1.75) {};
\node [] (51) at (0.0, -2.5) {};
\node [] (53) at (2.5, -1.75) {};
\node [] (54) at (2.5, -2.5) {};
\node [] (56) at (5.0, -0.75) {};
\node [] (57) at (5.0, -2.5) {};
\node [] (59) at (1.25, 0.5) {};
\node [] (60) at (1.25, -1.5) {};
\end{pgfonlayer}
\begin{pgfonlayer}{edgelayer}
\draw [-, fill={rgb,255: red,224; green,224; blue,224}, line width=1.0pt] (1.center) to (2.center) to (3.center) to (4.center) to (1.center);
\draw [-, fill={rgb,255: red,224; green,224; blue,224}, line width=1.0pt] (6.center) to (7.center) to (8.center) to (9.center) to (6.center);
\draw [-, fill={rgb,255: red,224; green,224; blue,224}, line width=1.0pt] (11.center) to (12.center) to (13.center) to (14.center) to (11.center);
\draw [-, fill={rgb,255: red,224; green,224; blue,224}, line width=1.0pt] (16.center) to (17.center) to (18.center) to (19.center) to (16.center);
\draw [-, fill={rgb,255: red,224; green,224; blue,224}, line width=1.0pt] (21.center) to (22.center) to (23.center) to (24.center) to (21.center);
\draw [in=90, out=-90, -, draw={rgb,255: red,156; green,84; blue,14}, line width=1.0pt] (26.center) to (27.center);
\draw [in=90, out=-90, -, draw={rgb,255: red,244; green,169; blue,64}, line width=1.0pt] (29.center) to (30.center);
\draw [in=90, out=-90, -, draw={rgb,255: red,156; green,84; blue,14}, line width=1.0pt] (32.center) to (33.center);
\draw [in=90, out=-90, -, draw={rgb,255: red,244; green,169; blue,64}, line width=1.0pt] (35.center) to (36.center);
\draw [in=90, out=-90, -, draw={rgb,255: red,156; green,84; blue,14}, line width=1.0pt] (38.center) to (39.center);
\draw [in=90, out=-90, -, draw={rgb,255: red,6; green,110; blue,226}, line width=1.0pt] (41.center) to (42.center);
\draw [in=90, out=-90, -, draw={rgb,255: red,244; green,169; blue,64}, line width=1.0pt] (44.center) to (45.center);
\draw [in=90, out=-90, -, draw={rgb,255: red,156; green,84; blue,14}, line width=1.0pt] (47.center) to (48.center);
\draw [in=90, out=-90, -, draw={rgb,255: red,156; green,84; blue,14}, line width=1.0pt] (50.center) to (51.center);
\draw [in=90, out=-90, -, draw={rgb,255: red,6; green,110; blue,226}, line width=1.0pt] (56.center) to (57.center);
\draw [in=90, out=-90, -, draw={rgb,255: red,244; green,169; blue,64}, line width=1.0pt] (53.center) to (54.center);
\draw [in=90, out=180, -, draw={rgb,255: red,244; green,169; blue,64}, line width=1.0pt, looseness=0.4118] (59.center) to (44.center);
\draw [in=90, out=0, -, draw={rgb,255: red,156; green,84; blue,14}, line width=1.0pt, looseness=0.4118] (59.center) to (38.center);
\draw [in=180, out=-90, -, draw={rgb,255: red,156; green,84; blue,14}, line width=1.0pt, looseness=0.4118] (33.center) to (59.center);
\draw [in=0, out=-90, -, draw={rgb,255: red,244; green,169; blue,64}, line width=1.0pt, looseness=0.4118] (36.center) to (59.center);
\draw [in=90, out=180, -, draw={rgb,255: red,156; green,84; blue,14}, line width=1.0pt, looseness=0.4118] (60.center) to (50.center);
\draw [in=90, out=0, -, draw={rgb,255: red,244; green,169; blue,64}, line width=1.0pt, looseness=0.4118] (60.center) to (53.center);
\draw [in=180, out=-90, -, draw={rgb,255: red,244; green,169; blue,64}, line width=1.0pt, looseness=0.4118] (45.center) to (60.center);
\draw [in=0, out=-90, -, draw={rgb,255: red,156; green,84; blue,14}, line width=1.0pt, looseness=0.4118] (48.center) to (60.center);
\end{pgfonlayer}
\begin{pgfonlayer}{labellayer}
\node (5) at (0, 2.5) {Alice};
\node  (10) at (2.5, 2.5) {music};
\node  (15) at (5.0, 2.5) {piano};
\node  (20) at (1.25, 1.5) {loves};
\node  (25) at (3.75, -0.5) {plays};
\end{pgfonlayer}
\end{tikzpicture}

\end{document}
