# Supplementary material for: Efficient Generation of Parameterised Quantum Circuits from Large Texts
Source: arXiv:2505.13208 source file (2025-05-19)
Supplement: Supplementary file 5 [file conj_rewritten_circuit.tex]

\documentclass{standalone}
\usepackage{tikz}

\begin{document}
\tikzset{every picture/.style={line width=0.75pt}} %set default line width to 0.75pt

\tikzstyle{gray_box}=[-, fill={rgb,255: red,224; green,224; blue,224}, line width=1.0pt]
\tikzstyle{fee1ba_box}=[-, fill={rgb,255: red,254; green,225; blue,186}, line width=1.0pt]
\tikzstyle{box}=[-, fill={rgb,255: red,255; green,255; blue,255}, line width=1.0pt]
\tikzstyle{9c540e_wire}=[-, draw={rgb,255: red,156; green,84; blue,14}, line width=1.0pt]
\tikzstyle{f4a940_wire}=[-, draw={rgb,255: red,244; green,169; blue,64}, line width=1.0pt]
\tikzstyle{066ee2_wire}=[-, draw={rgb,255: red,6; green,110; blue,226}, line width=1.0pt]
\tikzstyle{black_wire}=[-, draw={rgb,255: red,0; green,0; blue,0}, line width=1.0pt]

% When embedding into a *.tex file, uncomment and include the following lines:
\pgfdeclarelayer{nodelayer}
\pgfdeclarelayer{edgelayer}
\pgfdeclarelayer{labellayer}
\pgfsetlayers{nodelayer, edgelayer, labellayer}
\begin{tikzpicture}
	\begin{pgfonlayer}{nodelayer}
		\node [] (1) at (0.875, 3.25) {};
		\node [] (2) at (1.875, 3.25) {};
		\node [] (3) at (1.875, 3.75) {};
		\node [] (4) at (0.875, 3.75) {};
		\node [] (6) at (3.375, 3.25) {};
		\node [] (7) at (4.375, 3.25) {};
		\node [] (8) at (4.375, 3.75) {};
		\node [] (9) at (3.375, 3.75) {};
		\node [] (11) at (5.875, 3.25) {};
		\node [] (12) at (6.875, 3.25) {};
		\node [] (13) at (6.875, 3.75) {};
		\node [] (14) at (5.875, 3.75) {};
		\node [] (16) at (0.25, 0.75) {};
		\node [] (17) at (7.5, 0.75) {};
		\node [] (18) at (7.5, 2.5) {};
		\node [] (19) at (0.25, 2.5) {};
		\node [] (21) at (0.75, 1) {};
		\node [] (22) at (3.5, 1) {};
		\node [] (23) at (3.5, 2) {};
		\node [] (24) at (0.75, 2) {};
		\node [] (25) at (1.25, 1.25) {};
		\node [] (26) at (3, 1.25) {};
		\node [] (27) at (3, 1.75) {};
		\node [] (28) at (1.25, 1.75) {};
		\node [] (30) at (4.25, 1) {};
		\node [] (31) at (7, 1) {};
		\node [] (32) at (7, 2) {};
		\node [] (33) at (4.25, 2) {};
		\node [] (34) at (4.75, 1.25) {};
		\node [] (35) at (6.5, 1.25) {};
		\node [] (36) at (6.5, 1.75) {};
		\node [] (37) at (4.75, 1.75) {};
		\node [] (39) at (1.375, 3.25) {};
		\node [] (40) at (1.375, 2.5) {};
		\node [] (41) at (3.875, 3.25) {};
		\node [] (42) at (3.875, 2.5) {};
		\node [] (43) at (6.375, 3.25) {};
		\node [] (44) at (6.375, 2.5) {};
		\node [] (45) at (1.75, 2) {};
		\node [] (46) at (1.75, 1.75) {};
		\node [] (47) at (2.5, 2) {};
		\node [] (48) at (2.5, 1.75) {};
		\node [] (49) at (1.75, 1.25) {};
		\node [] (50) at (1.75, 1) {};
		\node [] (51) at (2.5, 1.25) {};
		\node [] (52) at (2.5, 1) {};
		\node [] (53) at (5.25, 2) {};
		\node [] (54) at (5.25, 1.75) {};
		\node [] (55) at (6, 2) {};
		\node [] (56) at (6, 1.75) {};
		\node [] (57) at (5.25, 1.25) {};
		\node [] (58) at (5.25, 1) {};
		\node [] (59) at (6, 1.25) {};
		\node [] (60) at (6, 1) {};
		\node [] (61) at (1.375, 0.75) {};
		\node [] (62) at (1.375, 0) {};
		\node [] (63) at (3.875, 0.75) {};
		\node [] (64) at (3.875, 0) {};
		\node [] (65) at (6.375, 0.75) {};
		\node [] (66) at (6.375, 0) {};
	\end{pgfonlayer}
	\begin{pgfonlayer}{edgelayer}
		\draw [style={gray_box}] (1.center)
			 to (2.center)
			 to (3.center)
			 to (4.center)
			 to cycle;
		\draw [style={gray_box}] (6.center)
			 to (7.center)
			 to (8.center)
			 to (9.center)
			 to cycle;
		\draw [style={gray_box}] (11.center)
			 to (12.center)
			 to (13.center)
			 to (14.center)
			 to cycle;
		\draw [style={fee1ba_box}] (16.center)
			 to (17.center)
			 to (18.center)
			 to (19.center)
			 to cycle;
		\draw [style=box] (21.center)
			 to (22.center)
			 to (23.center)
			 to (24.center)
			 to cycle;
		\draw [style={gray_box}] (25.center)
			 to (26.center)
			 to (27.center)
			 to (28.center)
			 to cycle;
		\draw [style=box] (30.center)
			 to (31.center)
			 to (32.center)
			 to (33.center)
			 to cycle;
		\draw [style={gray_box}] (34.center)
			 to (35.center)
			 to (36.center)
			 to (37.center)
			 to cycle;
		\draw [style={9c540e_wire}, in=90, out=-90] (39.center) to (40.center);
		\draw [style={f4a940_wire}, in=90, out=-90] (41.center) to (42.center);
		\draw [style={066ee2_wire}, in=90, out=-90] (43.center) to (44.center);
		\draw [style={black_wire}, in=90, out=-90] (45.center) to (46.center);
		\draw [style={black_wire}, in=90, out=-90] (47.center) to (48.center);
		\draw [style={black_wire}, in=90, out=-90] (49.center) to (50.center);
		\draw [style={black_wire}, in=90, out=-90] (51.center) to (52.center);
		\draw [style={black_wire}, in=90, out=-90] (53.center) to (54.center);
		\draw [style={black_wire}, in=90, out=-90] (55.center) to (56.center);
		\draw [style={black_wire}, in=90, out=-90] (57.center) to (58.center);
		\draw [style={black_wire}, in=90, out=-90] (59.center) to (60.center);
		\draw [style={9c540e_wire}, in=90, out=-90] (61.center) to (62.center);
		\draw [style={f4a940_wire}, in=90, out=-90] (63.center) to (64.center);
		\draw [style={066ee2_wire}, in=90, out=-90] (65.center) to (66.center);
	\end{pgfonlayer}
    \begin{pgfonlayer}{labellayer}
        \node [] (5) at (1.375, 3.5) {Alice};
		\node [] (10) at (3.875, 3.5) {music};
		\node [] (15) at (6.375, 3.5) {piano};
		\node [] (20) at (3.875, 2.25) {and};
		\node [] (29) at (2.125, 1.5) {loves};
		\node [] (38) at (5.6, 1.5) {plays};
    \end{pgfonlayer}
\end{tikzpicture}
\end{document}
