# Supplementary material for: Efficient Generation of Parameterised Quantum Circuits from Large Texts
Source: arXiv:2505.13208 source file (2025-05-19)
Supplement: Supplementary file 6 [file mergeBox.tex]

\documentclass{standalone}
\usepackage{tikz}

\begin{document}
\tikzset{every picture/.style={line width=0.75pt}} %set default line width to 0.75pt

\tikzstyle{gray_box}=[-, fill={rgb,255: red,224; green,224; blue,224}, line width=1.0pt]
\tikzstyle{box}=[-, fill={rgb,255: red,255; green,255; blue,255}, line width=1.0pt]
\tikzstyle{black_wire}=[-, draw={rgb,255: red,0; green,0; blue,0}, line width=1.0pt]
\tikzstyle{arrow}=[-{Stealth[length=5mm]}, draw={rgb,255: red,0; green,0; blue,0}, line width=2.0pt]

% When embedding into a *.tex file, uncomment and include the following lines:
\pgfdeclarelayer{nodelayer}
\pgfdeclarelayer{edgelayer}
\pgfdeclarelayer{labellayer}
\pgfsetlayers{nodelayer, edgelayer, labellayer}
\begin{tikzpicture}
	\begin{pgfonlayer}{nodelayer}
		\node [] (0) at (0.5, 4.5) {};
		\node [] (1) at (1.5, 4.5) {};
		\node [] (2) at (1.5, 5) {};
		\node [] (3) at (0.5, 5) {};
		\node [] (4) at (3, 4.5) {};
		\node [] (5) at (4, 4.5) {};
		\node [] (6) at (4, 5) {};
		\node [] (7) at (3, 5) {};
		\node [] (8) at (5.5, 4.5) {};
		\node [] (9) at (6.5, 4.5) {};
		\node [] (10) at (6.5, 5) {};
		\node [] (11) at (5.5, 5) {};
		\node [] (12) at (0.5, 3.5) {};
		\node [] (13) at (6.5, 3.5) {};
		\node [] (14) at (6.5, 4) {};
		\node [] (15) at (0.5, 4) {};
		\node [] (16) at (0.5, 2.5) {};
		\node [] (17) at (4, 2.5) {};
		\node [] (18) at (4, 3) {};
		\node [] (19) at (0.5, 3) {};
		\node [] (20) at (0.5, 1.5) {};
		\node [] (21) at (6.5, 1.5) {};
		\node [] (22) at (6.5, 2) {};
		\node [] (23) at (0.5, 2) {};
		\node [] (24) at (3, -0.5) {};
		\node [] (25) at (6.5, -0.5) {};
		\node [] (26) at (6.5, 0) {};
		\node [] (27) at (3, 0) {};
		\node [] (28) at (0.5, -2.5) {};
		\node [] (29) at (6.5, -2.5) {};
		\node [] (30) at (6.5, -2) {};
		\node [] (31) at (0.5, -2) {};
		\node [] (32) at (1, 4.5) {};
		\node [] (33) at (1, 4) {};
		\node [] (34) at (3.5, 4.5) {};
		\node [] (35) at (3.5, 4) {};
		\node [] (36) at (6, 4.5) {};
		\node [] (37) at (6, 4) {};
		\node [] (38) at (1, 3.5) {};
		\node [] (39) at (1, 3) {};
		\node [] (40) at (3.5, 3.5) {};
		\node [] (41) at (3.5, 3) {};
		\node [] (42) at (1, 2.5) {};
		\node [] (43) at (1, 2) {};
		\node [] (44) at (3.5, 2.5) {};
		\node [] (45) at (3.5, 2) {};
		\node [] (46) at (6, 3.5) {};
		\node [] (47) at (6, 2) {};
		\node [] (48) at (1, 1.5) {};
		\node [] (49) at (1, 1.25) {};
		\node [] (50) at (3.5, 1.5) {};
		\node [] (51) at (3.5, 1.25) {};
		\node [] (52) at (3.5, 0.25) {};
		\node [] (53) at (3.5, 0) {};
		\node [] (54) at (6, 1.5) {};
		\node [] (55) at (6, 0) {};
		\node [] (56) at (1, 0.25) {};
		\node [] (57) at (1, -0.75) {};
		\node [] (58) at (3.5, -0.5) {};
		\node [] (59) at (3.5, -0.75) {};
		\node [] (60) at (1, -1.75) {};
		\node [] (61) at (1, -2) {};
		\node [] (62) at (3.5, -1.75) {};
		\node [] (63) at (3.5, -2) {};
		\node [] (64) at (6, -0.5) {};
		\node [] (65) at (6, -2) {};
		\node [] (66) at (1, -2.5) {};
		\node [] (67) at (1, -3.25) {};
		\node [] (68) at (3.5, -2.5) {};
		\node [] (69) at (3.5, -3.25) {};
		\node [] (70) at (6, -2.5) {};
		\node [] (71) at (6, -3.25) {};
		\node [] (72) at (2.25, 0.75) {};
		\node [] (73) at (2.25, -1.25) {};
		\node [] (82) at (8, 1) {};
		\node [] (83) at (9, 1) {};
		\node [] (84) at (10.5, 5) {};
		\node [] (85) at (11.5, 5) {};
		\node [] (86) at (11.5, 5.5) {};
		\node [] (87) at (10.5, 5.5) {};
		\node [] (88) at (13, 5) {};
		\node [] (89) at (14, 5) {};
		\node [] (90) at (14, 5.5) {};
		\node [] (91) at (13, 5.5) {};
		\node [] (92) at (15.5, 5) {};
		\node [] (93) at (16.5, 5) {};
		\node [] (94) at (16.5, 5.5) {};
		\node [] (95) at (15.5, 5.5) {};
		\node [] (96) at (10.5, 4) {};
		\node [] (97) at (16.5, 4) {};
		\node [] (98) at (16.5, 4.5) {};
		\node [] (99) at (10.5, 4.5) {};
		\node [] (100) at (10.5, 3) {};
		\node [] (101) at (14, 3) {};
		\node [] (102) at (14, 3.5) {};
		\node [] (103) at (10.5, 3.5) {};
		\node [] (104) at (10.5, 2) {};
		\node [] (105) at (16.5, 2) {};
		\node [] (106) at (16.5, 2.5) {};
		\node [] (107) at (10.5, 2.5) {};
		\node [] (108) at (13, 0) {};
		\node [] (109) at (16.5, 0) {};
		\node [] (110) at (16.5, 0.5) {};
		\node [] (111) at (13, 0.5) {};
		\node [] (112) at (10.5, -2) {};
		\node [] (113) at (16.5, -2) {};
		\node [] (114) at (16.5, -1.5) {};
		\node [] (115) at (10.5, -1.5) {};
		\node [] (116) at (11, 5) {};
		\node [] (117) at (11, 4.5) {};
		\node [] (118) at (13.5, 5) {};
		\node [] (119) at (13.5, 4.5) {};
		\node [] (120) at (16, 5) {};
		\node [] (121) at (16, 4.5) {};
		\node [] (122) at (11, 4) {};
		\node [] (123) at (11, 3.5) {};
		\node [] (124) at (13.5, 4) {};
		\node [] (125) at (13.5, 3.5) {};
		\node [] (126) at (11, 3) {};
		\node [] (127) at (11, 2.5) {};
		\node [] (128) at (13.5, 3) {};
		\node [] (129) at (13.5, 2.5) {};
		\node [] (130) at (16, 4) {};
		\node [] (131) at (16, 2.5) {};
		\node [] (132) at (11, 2) {};
		\node [] (133) at (11, 1.75) {};
		\node [] (134) at (13.5, 2) {};
		\node [] (135) at (13.5, 1.75) {};
		\node [] (136) at (13.5, 0.75) {};
		\node [] (137) at (13.5, 0.5) {};
		\node [] (138) at (16, 2) {};
		\node [] (139) at (16, 0.5) {};
		\node [] (140) at (11, 0.75) {};
		\node [] (141) at (11, -0.25) {};
		\node [] (142) at (13.5, 0) {};
		\node [] (143) at (13.5, -0.25) {};
		\node [] (144) at (11, -1.25) {};
		\node [] (145) at (11, -1.5) {};
		\node [] (146) at (13.5, -1.25) {};
		\node [] (147) at (13.5, -1.5) {};
		\node [] (148) at (16, 0) {};
		\node [] (149) at (16, -1.5) {};
		\node [] (150) at (11, -2) {};
		\node [] (151) at (11, -2.75) {};
		\node [] (152) at (13.5, -2) {};
		\node [] (153) at (13.5, -2.75) {};
		\node [] (154) at (16, -2) {};
		\node [] (155) at (16, -2.75) {};
		\node [] (156) at (12.25, 1.25) {};
		\node [] (157) at (12.25, -0.75) {};
		\node [] (166) at (10.5, -3.25) {};
		\node [] (167) at (16.5, -3.25) {};
		\node [] (168) at (16.5, -2.75) {};
		\node [] (169) at (10.5, -2.75) {};
		\node [] (170) at (11, -2.75) {};
		\node [] (171) at (13.5, -2.75) {};
		\node [] (172) at (16, -2.75) {};
		\node [] (175) at (13.5, -3.25) {};
		\node [] (176) at (13.5, -4) {};
	\end{pgfonlayer}
	\begin{pgfonlayer}{edgelayer}
		\draw [style={gray_box}] (0.center) to (1.center) to (2.center) to (3.center) to cycle;
		\draw [style={gray_box}] (4.center) to (5.center) to (6.center) to (7.center) to cycle;
		\draw [style={gray_box}] (8.center) to (9.center) to (10.center) to (11.center) to cycle;
		\draw [style={gray_box}] (12.center) to (13.center) to (14.center) to (15.center) to cycle;
		\draw [style={gray_box}] (16.center) to (17.center) to (18.center) to (19.center) to cycle;
		\draw [style={gray_box}] (20.center) to (21.center) to (22.center) to (23.center) to cycle;
		\draw [style={gray_box}] (24.center) to (25.center) to (26.center) to (27.center) to cycle;
		\draw [style={gray_box}] (28.center) to (29.center) to (30.center) to (31.center) to cycle;
		\draw [style={black_wire}, in=90, out=-90] (32.center) to (33.center);
		\draw [style={black_wire}, in=90, out=-90] (34.center) to (35.center);
		\draw [style={black_wire}, in=90, out=-90] (36.center) to (37.center);
		\draw [style={black_wire}, in=90, out=-90] (38.center) to (39.center);
		\draw [style={black_wire}, in=90, out=-90] (40.center) to (41.center);
		\draw [style={black_wire}, in=90, out=-90] (42.center) to (43.center);
		\draw [style={black_wire}, in=90, out=-90] (44.center) to (45.center);
		\draw [style={black_wire}, in=90, out=-90] (46.center) to (47.center);
		\draw [style={black_wire}, in=90, out=-90] (48.center) to (49.center);
		\draw [style={black_wire}, in=90, out=-90] (50.center) to (51.center);
		\draw [style={black_wire}, in=90, out=-90] (52.center) to (53.center);
		\draw [style={black_wire}, in=90, out=-90] (54.center) to (55.center);
		\draw [style={black_wire}, in=90, out=-90] (56.center) to (57.center);
		\draw [style={black_wire}, in=90, out=-90] (58.center) to (59.center);
		\draw [style={black_wire}, in=90, out=-90] (60.center) to (61.center);
		\draw [style={black_wire}, in=90, out=-90] (62.center) to (63.center);
		\draw [style={black_wire}, in=90, out=-90] (64.center) to (65.center);
		\draw [style={black_wire}, in=90, out=-90] (66.center) to (67.center);
		\draw [style={black_wire}, in=90, out=-90] (68.center) to (69.center);
		\draw [style={black_wire}, in=90, out=-90] (70.center) to (71.center);
		\draw [style={black_wire}, in=90, out=180] (72.center) to (56.center);
		\draw [style={black_wire}, in=90, out=0] (72.center) to (52.center);
		\draw [style={black_wire}, in=180, out=-90] (49.center) to (72.center);
		\draw [style={black_wire}, in=0, out=-90] (51.center) to (72.center);
		\draw [style={black_wire}, in=90, out=180, looseness=0.75] (73.center) to (60.center);
		\draw [style={black_wire}, in=90, out=0, looseness=0.75] (73.center) to (62.center);
		\draw [style={black_wire}, in=180, out=-90] (57.center) to (73.center);
		\draw [style={black_wire}, in=0, out=-90] (59.center) to (73.center);
		\draw [style={arrow}, in=180, out=0] (82.center) to (83.center);
		\draw [style={gray_box}] (84.center) to (85.center) to (86.center) to (87.center) to cycle;
		\draw [style={gray_box}] (88.center) to (89.center) to (90.center) to (91.center) to cycle;
		\draw [style={gray_box}] (92.center) to (93.center) to (94.center) to (95.center) to cycle;
		\draw [style={gray_box}] (96.center) to (97.center) to (98.center) to (99.center) to cycle;
		\draw [style={gray_box}] (100.center) to (101.center) to (102.center) to (103.center) to cycle;
		\draw [style={gray_box}] (104.center) to (105.center) to (106.center) to (107.center) to cycle;
		\draw [style={gray_box}] (108.center) to (109.center) to (110.center) to (111.center) to cycle;
		\draw [style={gray_box}] (112.center) to (113.center) to (114.center) to (115.center) to cycle;
		\draw [style={black_wire}, in=90, out=-90] (116.center) to (117.center);
		\draw [style={black_wire}, in=90, out=-90] (118.center) to (119.center);
		\draw [style={black_wire}, in=90, out=-90] (120.center) to (121.center);
		\draw [style={black_wire}, in=90, out=-90] (122.center) to (123.center);
		\draw [style={black_wire}, in=90, out=-90] (124.center) to (125.center);
		\draw [style={black_wire}, in=90, out=-90] (126.center) to (127.center);
		\draw [style={black_wire}, in=90, out=-90] (128.center) to (129.center);
		\draw [style={black_wire}, in=90, out=-90] (130.center) to (131.center);
		\draw [style={black_wire}, in=90, out=-90] (132.center) to (133.center);
		\draw [style={black_wire}, in=90, out=-90] (134.center) to (135.center);
		\draw [style={black_wire}, in=90, out=-90] (136.center) to (137.center);
		\draw [style={black_wire}, in=90, out=-90] (138.center) to (139.center);
		\draw [style={black_wire}, in=90, out=-90] (140.center) to (141.center);
		\draw [style={black_wire}, in=90, out=-90] (142.center) to (143.center);
		\draw [style={black_wire}, in=90, out=-90] (144.center) to (145.center);
		\draw [style={black_wire}, in=90, out=-90] (146.center) to (147.center);
		\draw [style={black_wire}, in=90, out=-90] (148.center) to (149.center);
		\draw [style={black_wire}, in=90, out=-90] (150.center) to (151.center);
		\draw [style={black_wire}, in=90, out=-90] (152.center) to (153.center);
		\draw [style={black_wire}, in=90, out=-90] (154.center) to (155.center);
		\draw [style={black_wire}, in=90, out=180] (156.center) to (140.center);
		\draw [style={black_wire}, in=90, out=0] (156.center) to (136.center);
		\draw [style={black_wire}, in=180, out=-90] (133.center) to (156.center);
		\draw [style={black_wire}, in=0, out=-90] (135.center) to (156.center);
		\draw [style={black_wire}, in=90, out=180, looseness=0.75] (157.center) to (144.center);
		\draw [style={black_wire}, in=90, out=0, looseness=0.75] (157.center) to (146.center);
		\draw [style={black_wire}, in=180, out=-90, looseness=0.75] (141.center) to (157.center);
		\draw [style={black_wire}, in=0, out=-90] (143.center) to (157.center);
		\draw [style={gray_box}] (166.center) to (167.center) to (168.center) to (169.center) to cycle;
		\draw [style={black_wire}, in=90, out=-90] (175.center) to (176.center);
	\end{pgfonlayer}
    \begin{pgfonlayer}{labellayer}
		\node [] (74) at (1, 4.75) {Alice};
		\node [] (75) at (3.5, 4.75) {music};
		\node [] (76) at (6, 4.75) {piano};
		\node [] (77) at (3.5, 3.75) {and$_{top}$};
		\node [] (78) at (2.25, 2.75) {loves};
		\node [] (79) at (3.5, 1.75) {and$_{1}$};
		\node [] (80) at (4.75, -0.25) {plays};
		\node [] (81) at (3.5, -2.25) {and$_{bottom}$};
        \node [] (158) at (11, 5.25) {Alice};
		\node [] (159) at (13.5, 5.25) {music};
		\node [] (160) at (16, 5.25) {piano};
		\node [] (161) at (13.5, 4.25) {and$_{top}$};
		\node [] (162) at (12.25, 3.25) {loves};
		\node [] (163) at (13.5, 2.25) {and$_{1}$};
		\node [] (164) at (14.75, 0.25) {plays};
		\node [] (165) at (13.5, -1.75) {and$_{bottom}$};
        \node [] (179) at (13.5, -3) {MERGE};
		\node [] (180) at (13.65, -3.5) {t};
    \end{pgfonlayer}
\end{tikzpicture}
\end{document}
